# Supplementary material for: The 2022 n2c2/UW Shared Task on Extracting Social Determinants of Health
Source: arXiv:2301.05571 source file (2023-02-13)
Supplement: Supplementary file 1 [file literature_brainstorm.tex]

\documentclass{article}

\usepackage{geometry}
\geometry{letterpaper, portrait, margin=0.5in}

\usepackage[breaklinks]{hyperref}
\usepackage{url}

\usepackage[numbers, sort&compress]{natbib}
\usepackage{enumitem}
\usepackage[parfill]{parskip}
\bibliographystyle{unsrtnat}

\begin{document}

\section{To Review}

\citet{sheng2022nlp} - \textbf{need to download}, \textbf{need to review}

\section{SDOH in clinical text and NLP}

\subsection{Systematic reviews}

\citet{patra2021extracting} - \textbf{[CITE]} Review of SDOH work related to NLP. Good overview, including description of methodologies (lexicon, rule-based, supervised learning, etc.) Also includes overview of types of SDOH explored. 
\begin{itemize}[noitemsep,nolistsep]
    \item Rule-based approaches: 10, 12, 20, 21, 22, 26, 27, 28
    \item Supervised:
    \begin{itemize}[noitemsep,nolistsep]
        \item n-grams \& word embeddings: 29, 30, 31, 32, 33, 34, 35
        \item rule-based concepts as features: 17, 26, 38, 39
        \item Rule-based systems include UMLS and CTAKES : 36, 37
        \item discrete classifiers (SVM, RF, LR): 24, 29, 30, 32, 33, 34, 35, 37, 38, 40, 41, 42, 43, 44
        \item neural networks (CNN, FFNN, LSTM): 29, 32, 33, 42, 45, 46, 47
    \end{itemize}
\end{itemize}

\citet{bompelli2021social} - \textbf{[CITE]} Systematic review of SDOH in the EHR more broadly, not just NLP. NLP portion includes: rule-based methods, term expansion, topic modeling, and deep learning. Refers to two annotated corpora: Volig and Esta Bond [79] and SHAC

\subsubsection{Concept identification}

\citet{lowery2022using} - \textbf{[maybe CITE]} Explores the relationship between EMS transportation and SDOH using univariate and multivariate analyses. SDOH identified (extracted) using regular expressions. Describes detailed preprocessing (acronym expansion, spelling correction, lemmatization, etc.). Does not appear to present the performance of the regular expressions used. \textbf{DATA:} no description of annotated data set. 

\citet{hatef2019assessing} - \textbf{[CITE, Helpful for all authors to read.]} Explores problems of SDOH information in a large clinical data set, including structured data and unstructured text. SDOH are identified using rule-based approaches (linguistic patterns). Extraction of SDOH from text focuses on social connection, housing, and financial strain. Paper also include some analysis of structured representation of alcohol and tobacco use.\textbf{ DATA:} annotated 100 randomly selected notes for assessing goodness of rules, focusing on social connection, housing, and financial strain.

\citet{rouillard2022evaluation} - \textbf{ [optional CITE]} Rules-based approach for extracting SDOH information. Did not read thoroughly; however, probably can omit. \textbf{DATA:} unclear if annotated data created. 

\citet{bettencourt2020discovering} - SDOH concept identification, focused on identifying gaps in existing terminologies apologies. Used skip-n-gram model to identify domain specific and grams. \textbf{DATA:} does not appear to have annotated data

\subsection{Sentence or Note-level}

\citet{uzuner2008identifying} - the i2b2 NLP Smoking Challenge introduced a publicly available corpus where tobacco use status is labeled at the note-level. \textbf{DATA:} 502 annotated discharge summaries with note-level labels regarding smoking status

\citet{ gehrmann2018comparing} annotated MIMIC-III discharge summaries with note-level phenotype labels, including substance abuse and obesity. \textbf{DATA:} annotated 1610 notes with note-level phenotype labels that include SDOH: alcohol abuse and substance abuse. 

\citet{feller2018towards} annotated 38 different SDOH at the note-level. \textbf{DATA:} 3883 notes annotated at the note-level for sexual health-related SDOH, including gender, sexual orientation, sexual history, alcohol use, substance use, and housing status

\citet{han2022classifying} - \textbf{[CITE]} Created a annotated data set where 13 SDOH were annotated at the sentence-level as binary indicators. Explored rule-based approaches (e.g. cTAKES), discrete approaches (LRM RF), and deep learning approaches (CNN, LSTM, and BERT). SDOH predicted as text classification task, where each SDOH is a binary label (present versus absent). BERT performed the best of all methods. Experimentation included 8 of the 13 SDOH categories. \textbf{DATA:} annotation includes 3504 sentences from 2670 clinical notes for 13 SDOH at the sentence-level, including social environment, non-social, support circumstances/networks, substance abuse, housing, occupation, transportation.

\citet{yu2021study}  - Create corpus of 500 notes annotated with 5 SDOH concepts at document-level. Extracted concepts using BERT. \textbf{DATA:} 500 notes with document-level labels for 5 SDOH: gender, ethnicity, smoking, employment, and education.

\citet{yu2022assessing} -  Expansion of \citet{yu2021study}. Added 10 additional SDOH concepts (15 total concepts) to 500 annotated notes from prior work. Bert-based concept extraction as document-level. \textbf{DATA:} 500 notes with document-level labels for 15 SDOH: gender, alcohol, drug, marital status, education, occupation, smoking, race, ethnicity, language, physical activity, transportation, financial constraint, social cohesion, employment.

\citet{chapman2021rehoused} - Develop rule-based approach for identifying housing instability. Created small annotated data set with document-level labels associated with housing instability. \textbf{DATA:} 621 notes manually annotated for housing instability labels

\subsection{Relations and Events}

For example, \citet{wang2015automated} introduced a corpus with detailed substance use annotations for 691 clinical notes from the MTSamples website\footnote{MTSamples website: \url{http://www.mtsamples.com/}} DATA: 691 clinical notes annotated for substance use using relations annotations

\citet{wang2016investigating} - Builds on \citet{wang2015automated}, adding longitudinal analysis

\citet{Yetisgen2017substance} created detailed annotations for 13 SDOH in a publicly available corpus of 364 notes from the MTSamples website\footnote{MTSamples website: \url{http://www.mtsamples.com/}} that were created by human transcriptionists. 

\citet{reeves2021adaptation} - [CITE] - Introduces Moonstone, which is a rule-based NLP system for extracting social risk factors from clinical text. Moonstone utilizes term expansion that is based on semantic typing. \textbf{DATA:} 160 notes annotated for 8 SDOH concepts (social risk factors) with assertion values (present versus absent)

\section{Abstracts}

\citet{volij2020development} - Proposes SDOH annotation standard and annotate some notes; however, only an abstract.

\citet{hatef2021pilot} - \textbf{[OMIT, just abstract]}

\citet{dorr2019identifying} - Query determine expansion approach used to identify SDOH. Created annotated data set but detailed unclear. Just an abstract.

\section{Clinical text and NLP More Broadly}
\citet{demner2009can} - Broader description of how NLP can augment clinical decision-support systems. Includes review of NLP systems and history.

\section{EHR mining more broadly}
\citet{jensen2012mining} -  High-level survey describing the mining of EHR records, including clinical text (see page 398). Good overview of EHR data and relevant machine learning. Very high-level and probably not explicitly relevant to the SDOH paper. Includes citation regarding the heterogeneity of clinical text in ref 22 Meystre 2008.

\section{SDOH \& EHR (e.g. Case Studies)}

\citet{navathe2018hospital} - \textbf{[CITE]} Explores the prevalence of social factors in structured data and physician notes. The inclusion of text-encoded social factor information increased the prevalence of the social factors four tobacco use, alcohol abuse, drug abuse, depression, housing instability, fall risk, and poor social support.

\citet{chen2020social} - Review paper exploring SDOH data in the EHR and its impact on analysis and risk prediction. Work reviewing the introduction, which describes the conversion to electronic records and opportunity to enhance care delivery. Summarizes utility/usefulness of SDOH data. Does not appear to differentiate structured versus text SDOH data.

\citet{hatef2019public} - Relationship between patient SDOH and larger population-level community health record

\citet{wark2021engaging} -Focused on engaging stakeholders in the integration of SDOH information into the EHR. Relevant to Andrea and Serena's work.

\citet{cantor2018integrating} - Focused on the integration of SDOH information into the EHR. More policy and structure focused.

\bibliography{mybib}

\end{document}
