# Supplementary material for: The 2022 n2c2/UW Shared Task on Extracting Social Determinants of Health
Source: arXiv:2301.05571 source file (2023-02-13)
Supplement: Supplementary file 3 [file cover_letter_resubmit1.tex]

Kevin Lybarger
Assistant Professor
Department of Information Sciences and Technology
George Mason University
4400 University Dr. MSN 1G8
Fairfax, VA 22030
klybarge@gmu.edu


January 10, 2022


Dr. Suzanne Bakken
Editor-in-Chief
Journal of the American Medical Informatics Association


Dear Dr. Bakken,

I am pleased to resubmit the original research article entitled ``The 2022 n2c2/UW Shared Task on Extracting Social Determinants of Health'' for publication in the Journal of the American Medical Informatics Association Focus Issue on Social Determinants of Health (SDOH) Extraction.

This manuscript summarizes the National NLP Clinical Challenges (n2c2) extraction task, Track 2: Extracting Social Determinants of Health (n2c2/UW SDOH Challenge). We have carefully reviewed the reviewer feedback and updated the manuscript to address as many comments as possible. To address the review feedback, we included additional text and figures. Based on your approval, the manuscript word count is 4,499 (< 4,500 limit from email).

This manuscript has not been previously published and is not under consideration elsewhere. Dr. Özlem Uzuner, Dr Meliha Yetisgen, and I are co-editors on the JAMIA SDOH focus issue. We have no additional conflicts of interest to disclose. Thank you for your consideration.

Sincerely,

Kevin Lybarger
