# Supplementary material for: The 2022 n2c2/UW Shared Task on Extracting Social Determinants of Health
Source: arXiv:2301.05571 source file (2023-02-13)
Supplement: Supplementary file 4 [file response_document1.tex]

\documentclass[review, sort&compress]{elsarticle}

%\usepackage[letterpaper, portrait,  rmargin=2.0in]{geometry}
\usepackage[letterpaper, portrait, margin=1.0in]{geometry}
\usepackage{booktabs}

\usepackage[color=yellow,textwidth=1.5in,textsize=small]{todonotes}
\usepackage{xcolor}
\usepackage{hyperref}
\usepackage{soul}
%http://latexcolor.com/
\definecolor{comment_color}{rgb}{0.0, 0.18, 0.65}
\definecolor{internal_color}{rgb}{0.79, 0.0, 0.09}

\bibliographystyle{bst/elsarticle-num-names}
\AtBeginDocument{\colorlet{default_color}{.}}

\usepackage[parfill]{parskip}



\begin{document}

\noindent
{\huge Reviewer Response Document \par}
\bigskip

We carefully read the reviewer comments and have edited the manuscript to address as many points as possible. We interleaved our responses with the reviewers’ comments below, to provide context for the responses. A version of the manuscript indicating the associated changes is provided with the revised manuscript.


\section*{Reviewer: 1}

Comments to the Author

The authors contribute the overview paper for the n2c2/UW Shared NLP task on social determinants of health (SDoH). SDoH are impactful clinically, but we as a field do not do a good job at documenting SDoH, and when we do it is in free text clinical notes, which require NLP to be able to discern. Two corpora were created for this task (MIMIC-III and UW), and several experiments were run to discern internal (extraction) and external validity (generalizability, learning transfer). The tasks designed properly and I like the (appropriate) use of the paired bootstrap test to compare F1 measures. Many of the details for the corpora creation and contributing systems are found in companion manuscripts, but this meta-analysis is a necessary and valuable piece for reporting community tasks.

Minor Issues:


1. It would help if you could add 1 sentence describing the novel active learning framework method in terms of how it works, rather than jumping straight to its impact as you do currently on page 5 line ~line 50-52


\color{comment_color}
\textbf{RESPONSE:}  We added the following description of the active learning framework to the second paragraph of the Data subsection: 

    \begin{quote}
        ``The active learning framework selected batches for annotation based on diversity and informativeness. To assess diversity, samples were mapped into a vector space using TF-IDF weighted averages of pre-trained word embeddings. To assess informativeness, simplified note-level text classification tasks for substance use, employment, and living status were derived from the event annotations and used as a surrogate for event extraction. Sample informativeness was assessed as the entropy of note-level predictions for: \textit{Status Time} for \textit{Alcohol}, \textit{Drug}, and \textit{Tobacco}; \textit{Type Employ} for \textit{Employment}; and \textit{Status Living} for \textit{Living Status}. These labels capture normalized representations of social protective and risk factors.'' \\
\end{quote}

\color{default_color}    


Aesthetics:

1. I find the figures (3-8) depicting comparison of F1-measure results hard to digest in their present form. Part of the issue is that precision is a prevalence-based metric, which isn’t represented in Figure 3 at all, and incompletely represented in the remaining figures. I might suggest adding the total n in the title for each of the subgraphs (e.g., in figures 5+, Alcohol (n = ~2000), Living Status (n = ~1500); in figure 3 and 4, you could additionally add (n= ) under each label, e.g., Alcohol (n = \#), retired (n = \#). While this would be an improvement, I’m not entirely sold that this suggested visualization is necessarily ideal, as there may be alternative visualizations that convey the same (or more) information in a more optimum way.


\color{comment_color}
\textbf{RESPONSE:}  We appreciate the feedback regarding the error analysis figures. Below is a discussion for each figure:
\begin{itemize}
    \item Figure 3 was updated to include the number of gold events per event type for each subtask (e.g. ``Alcohol (n=308)'') and the average number of gold events per note. The average number of gold events per note was also added to allow comparison of the event type distribution across the subtasks.
    \item Figure 4 includes the average number of gold events by subtask and event type, to allow the prevalence of protective factors and risk factors to be compared across subtasks (e.g. Subtasks B and C have much higher prevalence of current drug use than Subtask A). The average gold event count was included instead of the absolute count, because the number of notes in each subtask varies.
    \item Figures 5-8 previously included the number of gold events per event density category (1, 2, 3+). These figures have been updated to also include the total number of events per event type in the subfigure titles (e.g. ``Alcohol (n=1,622)''). 
\end{itemize}

We updated the labels for the right-hand y-axes and legend labels so the terminologies are consistent within each figure and added a more descriptive caption to these figures. \\

\color{default_color}    

2. The Introduction then Background + Significance sections do not match the JAMIA Author Guidelines (Background, Significance, Objective).

\color{comment_color}
\textbf{RESPONSE:}  Based on the reviewer feedback and guidance from the Editor-in-Chief, we merged the previous Introduction and Background and Significance sections into a single Background and Significance section, removed the summary paragraph from the original Introduction, and added a brief Objective paragraph summarizing the significance and contributions of the paper. \\

%In our review of recent JAMIA publications, we found several papers that start with the headings Introduction and Methods and Materials\cite{king2022whom, eslami2022utilization, lokmic2022assessing, rahimi2022digital} and and papers that start with Introduction and then have paper-specific headings\cite{huang2020tutorial, kannampallil2023using}. Is it acceptable to keep the current paper organization (Introduction, Background and Significance, Methods and Materials, Results, Discussion, and Conclusions), or is reorganization of the initial sections needed? \\

\color{default_color}    


3. The last few sentences of the background SDOH Corpora (describing the n2c2/UW SDOH challenge and SHAC dataset) may flow better to start off the Materials and Methods Data subsection.  


\color{comment_color}
\textbf{RESPONSE:} The discussion of SHAC was removed from the discussion of existing SDOH corpora in the Related Work subsection and incorporated into the more detailed description of SHAC in the Data section. \\

\color{default_color}    


\section*{Reviewer: 2}

Comments to the Author

This paper presents the second track from the n2c2 NLP Challenge. This
track concerns three tasks about social determinants of health from
two distinct datasets of clinical notes (MIMIC-III database and the
annotated UW corpus), restricted to the social history section.

The authors present the corpora they used, the annotations provided
for the challenge, the way to compute evaluations of systems outputs,
and some issues existing between deidentified elements while they are
useful for a SDOH information extraction task.

From a point of view of presenting a challenge, the paper is well
written and presents all useful information concerning this SDOH
track.

I only have a basic remark: is it possible to give a few examples of
SDOH that were hard to identify for all systems? Currently, I have no
idea of how to explain why the top best systems did not achieve a
recall of 1. Are the missing information in the same category? Are
they composed of several terms? Are they rare SDOH?


\color{comment_color}
\textbf{RESPONSE:}  We expanded the error analysis to describe sources of error associated with the transition from the MIMIC data to the UW data (Subtask B) and present examples that remain difficult to classify even with MIMIC and UW training data (Subtask C). \\

\color{default_color}    



\section*{Reviewer: 3}

Comments to the Author

This paper describes a shared task for the extraction of social determinants of health from clinical notes. This work puts forward a dataset annotated for clinical information extraction and reviews a set of solutions for three specific tasks. The papers also describe the best-performing solutions and compare them based on evaluation metrics and systematic error analysis.

The paper is very well written. The main novelty of the work is the data resource and the analysis of models. This work provides insights into the information extraction task, is beneficial for the community, and opens new areas of research on this dataset and tasks.

I want to ask a few questions for clarification.

Line 48, page 4: This is the first time BRAT is mentioned in this paper. I suggest the link to the BRAT repository should be mentioned here as all readers might not be familiar with this tool.


\color{comment_color}
\textbf{RESPONSE:}  A sentence was added to the Data section indicating the BRAT annotation tool is online, including the relevant link as a footnote. \\
\color{default_color}    



line 48-50, page 5: what is the active selection framework used to select the training examples of the UW dataset? The criteria used for the reactive selection are unclear to me. Also, what are the metrics for measuring sample diversity and the prevalence of risk factors?


\color{comment_color}
\textbf{RESPONSE:}  We added a description of the active learning framework to the second paragraph of the Data subsection. The added text is included in response to Reviewer 1, comment 1. \\
 
\color{default_color}    



Line 20, page 8: what are the practical implications of these relaxations? For example, would the extracted information still be helpful in practice if a metric accepts a partial overlap?


\color{comment_color}
\textbf{RESPONSE:}  The relaxed scoring criteria is motivated by the utilization of the extracted information for secondary use. Trigger span equivalence is assessed using the described any overlap criteria, because the primary function of the trigger in the SHAC annotation scheme is to aggregate related arguments. The actual text of the trigger span, for example ``Tobacco use'' or ``smoking'', generally does not meaningfully add to the extracted representation of the patient SDOH. For labeled arguments, the subtype labels capture a normalized representation of the most relevant argument information. Other annotation schemes and annotated phenomena may warrant different scoring criteria. We updated the scoring description to include justification for the scoring criteria, including the relaxed trigger and labeled argument criteria. \\

\color{default_color}    


line 20, page 9: Is the linear layer the prediction layer attached to the BERT model or a hidden layer before the prediction layer?

\color{comment_color}
\textbf{RESPONSE:}  To improve clarity, the relevant sentences been updated to:
\begin{quote}
    ``Triggers were extracted as a sequence tagging task using BERT with a linear prediction layer at the output hidden states. '' \\
\end{quote}    

\color{default_color}    

It would be great if the authors could provide a quantitative metric of the computational cost of each of the solutions (e.g, training time, number of gpus, etc. ). Although large language models result in high performance, they can be too costly in terms of the computational cost and carbon footprint they generate. Since the best-performing model uses a T5 language model, I would like to know more about the computational cost and adaptability of such a system in a practical setting. 


\color{comment_color}
\textbf{RESPONSE:}  We agree that the computational cost associated with different extraction methodologies is interesting and quite important to the implementation of the designed systems. Participating teams submitted brief 2-page abstracts describing their systems, and we do not have access to information related to the hardware used, training time, energy consumption, etc. As each model was developed in different computational settings, directly comparing the computational cost is outside of the scope of the manuscript. \\

\color{default_color}    


%\bibliography{mybib}
%\bibliographystyle{acl_natbib}




\end{document}
